# Supplementary material for: First observation and branching fraction measurement of the $\Lambda_b^0\to D_s^- p$ decay
Source: arXiv:2212.12574 source file (2023-07-17)
Supplement: Supplementary file 1 [file supplementary-app.tex]

\clearpage

\section{CDS Supplementary material for LHCb-PAPER-2022-YYY}
\label{sec:Supplementary-App}

This appendix contains supplementary material that will be posted on the public CDS record but will not appear in the paper. \todo{Add as appendix}

Figure ~\ref{fig:pid-bach} shows invariant-mass distribution of $\LbDsP$ (left) and $\LbLcPi$ (right) candidates. The candidates are selected applying the full offline selection without the particle identification (PID) requirement on the companion track. This is represented as the filled orange ($\LbDsP$) and green ($\LbLcPi$) histograms. Candidates additionally passing or failing the PID requirements on the companion track are indicated by red circles and black squares, respectively.

\begin{figure}[htp]
    \centering
	\includegraphics[width=.475\textwidth]{figs-supp/pid_bach_lb2dsp_lab0_MassHypo_Dsp.pdf}
    \includegraphics[width=.475\textwidth]{figs-supp/pid_bach_lb2lcpi_lab0_MassFitConsD_M.pdf} 
	\caption{ The $m(\Dsm p)$ (left) and $m(\bar{\Lambda}_c^- \pi^+)$ invariant-mass distributions 
	after the full selection without the PID requirement 
	on the companion track (filled area) and passing (red circles)
	or failing (black squares) this selection.        
		}
    \label{fig:pid-bach}
\end{figure}

To estimate the contribution from the $D_s^-\pi^+$-like decays in the \BsDsK and \LbDsP data samples, an invariant-mass fit to the \BsDsPi, \DsKKPi sample under its own hypothesis is performed. The invariant-mass distribution of the \BsDsPi candidates is shown in Fig.~\ref{fig:bs2dspi}. 
The fit is composed of a signal modelled by the sum of a double-sided Hypatia function and a Johnson $S_U$ function, combinatorial background described by a single exponential and specific background components. Three different sources of specific background can be distinguished: 
the decays with the same final state as the signal ($\Bz\to\Dsm\pip$), 
the misidentified backgrounds (\BdDPi, \LbLcPi, \BsDsK) and 
the partially-reconstructed backgrounds which occur due to missing particles in the final state (\BdDsstPi, \BsDsstPi, \BsDsRho, \BsDsstRho). The shapes of specific backgrounds are taken from the simulated samples. 
The yields below 1\% of the signal component (\BsDsK, \BdDPi, \LbLcPi) are calculated from the branching fractions and efficiency predictions and are fixed in the fit. In the nominal data fit the signal's mean and width, the combinatorial background's slope and the yields are left free.

\begin{figure}[htp]
   \begin{center}
        \includegraphics[width=0.825\textwidth]{figs-supp/legend_Bs2DsPi.pdf}\\
        \includegraphics[width=0.49\textwidth]{figs-supp/mdfit_beautymass_Bs2DsPi_lin.pdf}
        \includegraphics[width=0.49\textwidth]{figs-supp/mdfit_beautymass_Bs2DsPi_log.pdf}
    \end{center}
	\caption{Invariant-mass distribution of $\BsDsPi$ candidates, in (left) linear and (right) logarithmic scale, where the signal and background contributions are overlaid. The individual components of the fit are illustrated in the legend.}
	\label{fig:bs2dspi}
\end{figure}

The contribution from the $D_s^\mp  K^\pm$-like decays in the \LbDsP data sample is estimated from an invariant-mass fit to the \BsDsK sample under its own hypothesis. The invariant-mass distribution of the \BsDsK candidates is shown in Fig.~\ref{fig:bs2dsk}. The fit is composed of a signal modelled by the sum of a double-sided Hypatia function and a Johnson $S_U$ function, combinatorial background described by a single exponential and specific background components.
Unlike in the \BsDsPi sample, 
four different sources of background for \BsDsK signal can be distinguished: 
the decays with the same final state as the signal ($\Bz\to\Dsm\Kp$), 
the partially-reconstructed backgrounds which occur due to missing particles in the final state (\BdDsstK, \BsDsstK, \BsDsKst, \BsDsstKst), 
the misidentified backgrounds (\BsDsPi, \LbDsP) and 
the backgrounds that are both partially reconstructed and misidentified (\BsDsstPi, \BsDsRho, \BsDsstRho, \LbDsstP). 
To improve the stability of the fit, 
the contributions from the suppressed \BsDsPilike decays are fixed using the fit to \BsDsPi candidates,
while the remaining yields of the \BdDPi, \BdDK, \LbLcPi and \LbLcK are calculated from their branching fractions
and relative efficiencies. In the nominal data fit the signal's mean and width, the combinatorial background's slope and the yields are left free. 

\begin{figure}[htp]
   \begin{center}
        \includegraphics[width=0.99\textwidth]{figs-supp/legend_Bs2DsK.pdf}\\
        \includegraphics[width=0.49\textwidth]{figs-supp/mdfit_beautymass_Bs2DsK_lin.pdf}
        \includegraphics[width=0.49\textwidth]{figs-supp/mdfit_beautymass_Bs2DsK_log.pdf}
    \end{center}
	\caption{Invariant-mass distribution of $\BsDsK$ candidates, in (left) linear and (right) logarithmic scale, where the signal and background contributions are overlaid. The individual components in the fit are illustrated in the legend.}
	\label{fig:bs2dsk}
\end{figure}

The selection of candidates is divided into several stages. First, the particles must be inside of the LHCb detector acceptance. Afterwards, they proceed through two steps of the trigger selection: hardware and software. Candidates which pass these stages are subject to a further loose preselection. Finally, the selected candidates are further required to fulfil the kinematic, geometric and particle identification requirements. The total efficiency of selection is split into these stages. Table ~\ref{tab:eff-total} shows the ratio of the selection efficiencies divided into the categories mentioned above.

\begin{table}[htbp]
\small
\centering
\begin{footnotesize} 
\caption{A breakdown of the relative efficiency ratios of the \LbLcPi and \LbDsP decays.}
\label{tab:eff-total}
\begin{tabular}{lc}
  \toprule
	Requirement      & Ratio $\epsilon(\LbLcPi)$/$\epsilon(\LbDsP)$  \\
	\midrule 
	LHCb acceptance           & $0.9625 \pm 0.0016$ \\
	Hardware trigger          &  $0.995 \pm 0.006$  \\
	Software trigger and preselection &  $1.1370 \pm 0.0026$ \\
	Kinematic and geometric selection &  $0.7580 \pm 0.0018$ \\
	Particle identification selection &  $1.278 \pm 0.005$  \\
	\midrule
	Total                     &  $\EffRatioLbLcPiLbDsp$ \\
  \bottomrule

\end{tabular}
\end{footnotesize} 
\end{table} 

Table~\ref{tab:sys:tot:lb2dsp} summarises the invariant-mass fit systematic uncertainties possibly affecting the measurement which are discussed in Sect.~\ref{sec:systematics} of the paper. 

\begin{table}[htp]
    \small
    \centering
    \footnotesize
    \caption{Summary of the invariant-mass fit systematic uncertainties possibly affecting the measurement, presented as percentage of the branching fraction of $\LbDsP$ and $\LbLcPi$ respectively.}
    \label{tab:sys:tot:lb2dsp}
    \begin{tabular}{lcc}
    \toprule
        Source           & $\LbDsP$ sample & $\LbLcPi$ sample \\
    \midrule
    Signal parametrisation: & 0.54\% & 0.27\% \\
	Combinatorial background parametrisation: & 0.73\% & 0.04\%\\
	Constrained/fixed yields: & 0.71\% & 0.03\% \\
	Specific background parametrisation: & 0.89\% & 0.01\% \\
	\midrule
	Total: & 1.46\%  & 0.28\%\\
    \bottomrule
    \end{tabular}
\end{table}

\clearpage
